# Supplementary material for: Distilling Information Reliability and Source Trustworthiness from Digital Traces
Source: arXiv:1610.07472 source file (2017-04-02)
Supplement: Supplementary file 1 [file 070appendix.tex]

% \xhdr{Evaluation inference with L1 regularization}

%To simplify the derivation we assume there is a single topic, the extension to multiple topics is trivial. We further assume $K(t) = \int^t_0 k(t) \, ds$.
%\begin{align*}
%\Lcal &=
%  \sum_{d=1}^{|\Dcal | } \sum_{i: e_i \in \Hcal_d(T)} \log p(\Delta_i | t_i, \betab_d, \{
%\alphab_s\}_{s=1}^{|\Scal |}, \mathbf{w}_d) - \eta \betab \\
%
%  & \quad \sum_{d=1}^{|\Dcal | } \sum_{\substack{i: e_i \in \Hcal_d(T) \\ \tau_i < T}} \log (\sum_j \beta_{d_{i, j}}  k(\tau_i-t_j) + \alpha_{s_i})\\
%
%  &\quad -\sum_{i: e_i \in \Hcal_d(T)} \sum_j \beta_{d_{i, j}}\big(K(T-t_j) -K(t_i-t_j)\big)\\
%  &\quad \quad \quad - \alpha_{s_i}(T-t_i) - \eta \betab\\
%
%\end{align*}
%Using Jensen inequality and assuming $\sum_j \zeta_{i,j} + \zeta_{i,J+1} =1$:
%\begin{align*}
%\Lcal&<
%  \sum_{d=1}^{|\Dcal | } \sum_{\substack{i: e_i \in \Hcal_d(T) \\ \tau_i < T}} \sum_j \zeta_{i,j} \log (\beta_{d_{i, j}}) + \zeta_{i,j}\log(k(\tau_i-t_j))\\
%  &\quad \quad \quad \quad \quad + \zeta_{i,J+1} \log(\alpha_{s_i})\\
%  &\quad -\sum_{i: e_i \in \Hcal_d(T)} \sum_j \beta_{d_{i, j}}\big(K(T-t_j) -K(t_i-t_j)\big)\\
%  &\quad \quad \quad - \alpha_{s_i}(T-t_i) - \eta \betab\\
%\end{align*}

%We can now maximize this lower bound with respect to parameters $\betab, \alphab$ and $\zeta$ by using Lagrange multipliers we derive following update rules:

%\begin{align*}
%  j \leq J:& \zeta_{i,j} = \frac{\beta_{d_{i, j}}}{\sum_j \beta_{d_{i, j}}  k(\tau_i-t_j) + \alpha_{s_i}}\\
%  j = J+1:&\zeta_{i,j} = \frac{\alpha_{s_i}}{\sum_j \beta_{d_{i, j}}  k(\tau_i-t_j) + \alpha_{s_i}}
%\end{align*}

%\begin{align*}
%   \beta_{d, j} &= \frac{\sum_{\substack{i: e_i \in \Hcal_d(T) \\ \tau_i < T}}  \zeta_{i, j}}{  \sum_{i: e_i \in \Hcal_d(T)} \big(K(\tau_i-t_j) -K(t_i-t_j)\big) + \eta}\\
%   \alpha_{s} &= \frac{\sum_{d=1}^{|\Dcal |} \sum_{\substack{i: e_i \in \Hcal_d(T) \\ s_i=s,\tau_i < T}}  \zeta_{i, J+1}}{\sum_{d=1}^{|\Dcal |} \sum_{\substack{i: e_i \in \Hcal_d(T) \\ s_i=s}}
%(\tau_i -t_i)}
% \end{align*}
%
% \setlength\tabcolsep{3pt}
% \begin{tabular}{c c c c c c c|c c c c c c c }
%   \hhline{======|======|======}
%   \multicolumn{2}{c}{domain}&\multicolumn{2}{c}{\#links}&\multicolumn{2}{c|}{T remove}&\multicolumn{2}{c|}{follow-up links}  & \multicolumn{2}{c}{domain}&\multicolumn{2}{c}{\#links}&\multicolumn{2}{c|}{T remove}&\multicolumn{2}{c|}{follow-up links}  &
%    \hhline{------|------|------}
%   % %
%    \multicolumn{2}{c}{wikipedia.org} &
%    \multicolumn{2}{c}{19K} &
%    \multicolumn{2}{c |}{239d} &
%
%    \multicolumn{2}{c}{wikipedia.org}&
%    \multicolumn{2}{c}{20K}&
%    \multicolumn{2}{c |}{330d} &
%
%    \multicolumn{2}{c}{103154}&
%    \multicolumn{2}{c}{top 0.06\%} &
%    \multicolumn{2}{c}{12h} \\
%
%    \multicolumn{2}{c}{twitter.com} &
%    \multicolumn{2}{c}{11K} &
%    \multicolumn{2}{c |}{2y} &
%
%    \multicolumn{2}{c}{youtube.com}&
%    \multicolumn{2}{c}{11K}&
%    \multicolumn{2}{c |}{$>100$y} &
%
%    \multicolumn{2}{c}{103154}&
%    \multicolumn{2}{c}{top 0.06\%} &
%    \multicolumn{2}{c}{12h} \\
%
%    \multicolumn{2}{c}{facebook.com} &
%    \multicolumn{2}{c}{10K} &
%    \multicolumn{2}{c|}{$2$y} &
%
%    \multicolumn{2}{c}{cia.gov}&
%    \multicolumn{2}{c}{14K}&
%    \multicolumn{2}{c|}{$14$y} &
%
%    \multicolumn{2}{c}{84651}&
%    \multicolumn{2}{c}{top 0.05\%}&
%    \multicolumn{2}{c}{2.8y} \\
%   % %
%
%    \multicolumn{2}{c}{guardian.co.uk} &
%    \multicolumn{2}{c}{12K} &
%    \multicolumn{2}{c|}{$>100$y} &
%
%    \multicolumn{2}{c}{abc.net.au}&
%    \multicolumn{2}{c}{10K}&
%    \multicolumn{2}{c|}{$>100$y} &
%
%    \multicolumn{2}{c}{84651}&
%    \multicolumn{2}{c}{top 0.05\%}&
%    \multicolumn{2}{c}{2.8y} \\
%
%    \hhline{------|------|------}
%   % %
%   % %\multicolumn{2}{c |}{100 - 3000	} & \multicolumn{2}{c |}{3955 - 68816} & \multicolumn{2}{c }{4000 - 10k} \\
%    \hhline{------|------|------}
%    \multicolumn{2}{c}{999*}&
%    \multicolumn{2}{c}{1.5K}&
%    \multicolumn{2}{c|}{$3$mi} &
%
%    \multicolumn{2}{c}{windclub.org}&
%    \multicolumn{2}{c}{1.4K} &
%    \multicolumn{2}{c|}{1mi} &
%
%    \multicolumn{2}{c}{364001}&
%    \multicolumn{2}{c}{top 0.80\%}&
%    \multicolumn{2}{c}{8h} \\
%
%    \multicolumn{2}{c}{drown*\footnotemark}&
%    \multicolumn{2}{c}{1.1K}&
%    \multicolumn{2}{c|}{$>100$y} &
%
%    \multicolumn{2}{c}{basket*\footnotemark}&
%    \multicolumn{2}{c}{3k}&
%    \multicolumn{2}{c|}{$>100$y} &
%
%    \multicolumn{2}{c}{53013}&
%    \multicolumn{2}{c}{top 0.03\%}&
%    \multicolumn{2}{c}{80y} \\
%
%    \hhline{------|------|------}
%    \multicolumn{2}{c}{6668886.com}&
%    \multicolumn{2}{c}{27}&
%    \multicolumn{2}{c|}{$1$mi} &
%
%    \multicolumn{2}{c}{free*\footnotemark}&
%    \multicolumn{2}{c}{20} &
%    \multicolumn{2}{c|}{1mi} &
%
%    \multicolumn{2}{c}{148722}&
%    \multicolumn{2}{c}{top 3.0\%}&
%    \multicolumn{2}{c}{9.5h} \\
%
%    \multicolumn{2}{c}{sabian.com}&
%    \multicolumn{2}{c}{1.1K}&
%    \multicolumn{2}{c|}{$>100$y} &
%
%    \multicolumn{2}{c}{russia-today.ru}&
%    \multicolumn{2}{c}{100}&
%    \multicolumn{2}{c|}{$>100$y} &
%
%    \multicolumn{2}{c}{27020}&
%    \multicolumn{2}{c}{top 0.87\%}&
%    \multicolumn{2}{c}{$>100$y} \\
%   %
%    \hhline{------|------|------}
%    \multicolumn{2}{c}{bij.pl}&
%    \multicolumn{2}{c}{111}&
%    \multicolumn{2}{c|}{$<1$mi} &
%
%    \multicolumn{2}{c}{web*\footnotemark}&
%    \multicolumn{2}{c}{65}&
%    \multicolumn{2}{c|}{1mi}&
%
%    \multicolumn{2}{c}{401835}&
%    \multicolumn{2}{c}{top 3.0\%}&
%    \multicolumn{2}{c}{8.0h} \\
%
%    \multicolumn{2}{c}{motley.com}&
%    \multicolumn{2}{c}{32}&
%    \multicolumn{2}{c|}{$>100$y} &
%
%    \multicolumn{2}{c}{iwojima.com}&
%    \multicolumn{2}{c}{30}&
%    \multicolumn{2}{c|}{$>100$y} &
%
%    \multicolumn{2}{c}{173677}&
%    \multicolumn{2}{c}{top 2\%}&
%    \multicolumn{2}{c}{$>100$y} \\
% % % onesixthwarriors.com(39) & lost-in-france.com(69 links) & 75245 (top 0.75\%)\\
% % %
% % %\multicolumn{2}{c |}{40 - 100} & \multicolumn{2}{c |}{3955 - 68816} & \multicolumn{2}{c }{4000 - 10k} \\
% % \hhline{--|--|--}
% % \multicolumn{2}{c |}{cisco.com-1-$<1$ mi}&
% % \multicolumn{2}{c |}{familychristian.com-1-$<1$mi} &
% % \multicolumn{2}{c }{401835-top 3\%-8h ) } \\
% % \multicolumn{2}{c |}{animati*\footnotemark-4-$>100$y}&
% % \multicolumn{2}{c |}{thetech.org-6-$>100$y} &
% % \multicolumn{2}{c }{173677-top 2\%-$>100$y} \\
% % shakespeareauthorship.com(33) & iraqigovernment.org(41 links) & 75699 (top 4\%)\\
% \end{tabular}
